# Supplementary material for: Accurate Prediction of Core Level Binding Energies from Ground-State Density Functional Calculations: The Importance of Localization and Screening
Source: arXiv:2406.06345 ancillary file (2024-06-10)
Supplement: Supplementary file 1 [file SI.pdf]

# Supporting Information: Accurate Prediction of Core Level Binding Energies from Ground-State Density Functional Calculations: The Importance of Localization and Screening

Jincheng Yu,[†] Yuncai Mei,[†] Zehua Chen,[†,‡] and Weitao Yang[*,†,¶]

†*Department of Chemistry, Duke University, Durham, NC 27708, USA*

‡*Theoretical Chemistry Institute and Department of Chemistry, University of Wisconsin-Madison, Madison, WI 53706, USA*

¶*Department of Physics, Duke University, Durham, NC 27708, USA*

E-mail: weitao.yang@duke.edu

Table S1: Absolute core-level binding energies (CLBEs) of systems from CORE65 test set.[S1] The calculations were performed with def2-TZVP/BLYP using QM4D.[S2]

| index | mol | core level | Ref. | orbital | DFA | GSC2 | GSC | LOSC2 | lrLOSC |
|---|---|---|---|---|---|---|---|---|---|
| 1 | methane | C1s | 290.84 | 0 | 269.23 | 293.80 | 299.83 | 299.83 | 293.80 |
| 2 | ethane | C1s | 290.71 | 0 1 | 269.36 | 283.29 | 282.08 | 299.97 | 293.68 |
| 3 | ethene | C1s | 290.82 | 0 1 | 269.71 | 284.03 | 282.77 | 300.31 | 293.82 |
| 4 | ethyne | C1s | 291.25 | 0 1 | 269.91 | 284.64 | 283.26 | 300.51 | 294.23 |
| 5 | carbonmonoxide | O1s | 542.1 | 0 | 513.87 | 547.51 | 556.30 | 556.30 | 545.87 |
| 5 | carbonmonoxide | C1s | 296.23 | 1 | 272.87 | 298.84 | 303.43 | 303.43 | 298.93 |
| 6 | carbondioxide | O1s | 541.32 | 0 1 | 513.18 | 545.97 | 555.20 | 555.53 | 544.66 |
| 6 | carbondioxide | C1s | 297.7 | 2 | 274.61 | 300.28 | 305.19 | 305.19 | 300.36 |
| 7 | tetrafluoromethane | F1s | 695.2 | 0 1 2 3 | 662.63 | 698.47 | 709.51 | 709.52 | 698.48 |
| 7 | tetrafluoromethane | C1s | 301.9 | 4 | 278.87 | 304.45 | 309.50 | 309.50 | 304.45 |
| 8 | fluoromethane | F1s | 692.4 | 0 | 660.30 | 695.97 | 707.19 | 707.19 | 695.97 |
| 8 | fluoromethane | C1s | 293.56 | 1 | 271.65 | 296.48 | 302.26 | 302.26 | 296.48 |
| 9 | trifluoromethane | F1s | 694.1 | 0 1 2 | 661.96 | 697.63 | 708.82 | 708.85 | 697.65 |
| 9 | trifluoromethane | C1s | 299.16 | 3 | 276.49 | 301.86 | 307.12 | 307.12 | 301.86 |
| 10 | methanol | O1s | 538.88 | 0 | 510.88 | 544.09 | 553.44 | 553.44 | 542.38 |
| 10 | methanol | C1s | 292.3 | 1 | 270.80 | 295.43 | 301.43 | 301.43 | 295.42 |
| 11 | formaldehyde | O1s | 539.33 | 0 | 511.54 | 544.47 | 554.02 | 554.03 | 542.76 |
| 11 | formaldehyde | C1s | 294.38 | 1 | 272.44 | 297.46 | 303.03 | 303.03 | 297.52 |
| 12 | dimethylether | O1s | 538.36 | 0 | 511.00 | 543.55 | 553.46 | 553.46 | 541.91 |
| 12 | dimethylether | C1s | 292.17 | 1 2 | 270.78 | 295.19 | 301.38 | 301.39 | 295.20 |
| 13 | formicacid | O1s(OH) | 540.69 | 0 | 512.73 | 545.64 | 555.22 | 555.22 | 543.98 |
| 13 | formicacid | O1s(C=O) | 539.02 | 1 | 511.19 | 543.86 | 553.69 | 553.69 | 542.17 |
| 13 | formicacid | C1s | 295.75 | 2 | 273.47 | 298.49 | 304.06 | 304.06 | 298.57 |
| 14 | acetone | O1s | 537.73 | 0 | 510.62 | 542.88 | 553.08 | 553.08 | 541.18 |
| 14 | acetone | C1s(C=O) | 293.88 | 1 | 272.10 | 296.53 | 302.69 | 302.69 | 296.58 |
| 14 | acetone | C1s(CH3) | 291.23 | 2 3 | 269.90 | 293.76 | 299.95 | 300.51 | 294.11 |
| 15 | methylformate | O1s(OCH3) | 539.64 | 0 | 512.52 | 544.86 | 554.95 | 554.95 | 543.25 |
| 15 | methylformate | O1s(C=O) | 538.24 | 1 | 510.93 | 543.39 | 553.41 | 553.41 | 541.70 |
| 16 | aceticacid | O1s(OH) | 540.1 | 0 | 512.35 | 545.05 | 554.83 | 554.83 | 543.40 |
| 16 | aceticacid | O1s(C=O) | 538.31 | 1 | 510.72 | 543.15 | 553.21 | 553.21 | 541.47 |
| 16 | aceticacid | C1s(COOH) | 295.35 | 2 | 273.30 | 298.03 | 303.90 | 303.90 | 298.10 |

TABLE S1 continued:

| index | mol | core level | Ref. | orbital | DFA | GSC2 | GSC | LOSC2 | lrLOSC |
|---|---|---|---|---|---|---|---|---|---|
| 16 | aceticacid | C1s(CH3) | 291.55 | 3 | 270.17 | 294.53 | 300.80 | 300.80 | 294.52 |
| 17 | water | O1s | 539.7 | 0 | 510.94 | 544.88 | 553.64 | 553.64 | 543.11 |
| 18 | ozone | O1smiddle | 546.44 | 0 | 518.76 | 551.86 | 561.12 | 561.12 | 550.37 |
| 18 | ozone | O1sterminal | 541.75 | 1 2 | 514.11 | 533.69 | 530.78 | 556.60 | 545.09 |
| 19 | oxygen | O1sweaker | 544.2 | 0 | 514.86 | 536.45 | 534.48 | 557.31 | 547.24 |
| 19 | oxygen | O1sstronger | 543.1 | 1 | 514.86 | 536.45 | 534.47 | 557.31 | 547.24 |
| 20 | nitrogen | N1s | 409.93 | 0 1 | 383.94 | 401.83 | 399.41 | 419.97 | 413.05 |
| 21 | ammonia | N1s | 405.52 | 0 | 380.62 | 408.77 | 416.66 | 416.66 | 408.77 |
| 22 | hydrogencyanide | N1s | 406.8 | 0 | 381.89 | 409.93 | 417.93 | 417.93 | 409.93 |
| 22 | hydrogencyanide | C1s | 293.5 | 1 | 271.22 | 296.34 | 301.81 | 301.81 | 296.34 |
| 23 | acetonitrile | N1s | 405.58 | 0 | 381.13 | 408.70 | 417.16 | 417.16 | 408.70 |
| 23 | acetonitrile | C1s(CH3) | 292.88 | 1 | 271.19 | 295.68 | 301.79 | 301.80 | 295.68 |
| 23 | acetonitrile | C1s(CN) | 292.6 | 2 | 270.80 | 295.60 | 301.39 | 301.39 | 295.60 |
| 24 | glycine | O1s(OH) | 540.2 | 0 | 512.43 | 545.08 | 554.89 | 554.89 | 543.43 |
| 24 | glycine | O1s(C=O) | 538.4 | 1 | 510.91 | 543.24 | 553.39 | 553.39 | 541.56 |
| 24 | glycine | N1s | 405.4 | 2 | 380.99 | 408.63 | 417.04 | 417.04 | 408.63 |
| 24 | glycine | C1s(COOH) | 295.2 | 3 | 273.24 | 297.82 | 303.83 | 303.83 | 297.89 |
| 24 | glycine | C1s(CH2) | 292.3 | 4 | 270.97 | 295.20 | 301.60 | 301.60 | 295.19 |
| 25 | pyridine | N1s | 404.82 | 0 | 381.12 | 407.90 | 417.16 | 417.16 | 407.90 |
| 26 | pyrrole | N1s | 406.18 | 0 | 382.35 | 409.34 | 418.39 | 418.39 | 409.34 |
| 27 | aniline | N1s | 405.31 | 0 | 381.43 | 408.40 | 417.47 | 417.46 | 408.40 |
| 28 | urea | O1s | 537.19 | 0 | 509.78 | 542.04 | 552.27 | 552.27 | 540.32 |
| 28 | urea | N1s | 406.09 | 1 2 | 381.72 | 409.22 | 417.77 | 417.77 | 409.23 |
| 28 | urea | C1s | 294.84 | 3 | 272.89 | 297.60 | 303.49 | 303.49 | 297.64 |
| 29 | methylamine | N1s | 405.17 | 0 | 380.62 | 408.37 | 416.66 | 416.66 | 408.37 |
| 31 | benzene | C1s | 290.38 | 0 1 2 3 4 5 | 269.77 | 277.42 | 273.13 | 300.37 | 293.28 |

Table S2: Absolute CLBEs of systems from CORE65 test set.[S1] The calculations were performed with def2-TZVP/B3LYP using QM4D.[S2]

| index | mol | core level | Ref. | orbital | DFA | GSC2 | GSC | LOSC2 | lrLOSC |
|---|---|---|---|---|---|---|---|---|---|
| 1 | methane | C1s | 290.84 | 0 | 276.46 | 293.60 | 300.96 | 300.96 | 293.60 |

TABLE S2 continued:

| index | mol | core level | Ref. | orbital | DFA | GSC2 | GSC | LOSC2 | lrLOSC |
|---|---|---|---|---|---|---|---|---|---|
| 2 | ethane | C1s | 290.71 | 0 1 | 276.61 | 286.36 | 286.79 | 301.11 | 293.49 |
| 3 | ethene | C1s | 290.82 | 0 1 | 276.99 | 287.08 | 287.45 | 301.49 | 293.65 |
| 4 | ethyne | C1s | 291.25 | 0 1 | 277.23 | 287.66 | 287.91 | 301.72 | 294.10 |
| 5 | carbonmonoxide | O1s | 542.1 | 0 | 523.60 | 546.87 | 557.72 | 557.72 | 545.27 |
| 5 | carbonmonoxide | C1s | 296.23 | 1 | 280.29 | 298.90 | 304.75 | 304.75 | 299.00 |
| 6 | carbondioxide | O1s | 541.32 | 0 1 | 522.99 | 536.85 | 536.27 | 557.03 | 544.16 |
| 6 | carbondioxide | C1s | 297.7 | 2 | 282.27 | 300.63 | 306.73 | 306.73 | 300.71 |
| 7 | tetrafluoromethane | F1s | 695.2 | 0 1 2 3 | 673.65 | 686.62 | 686.76 | 711.17 | 697.89 |
| 7 | tetrafluoromethane | C1s | 301.9 | 4 | 286.54 | 304.81 | 311.07 | 311.07 | 304.81 |
| 8 | fluoromethane | F1s | 692.4 | 0 | 671.17 | 695.17 | 708.70 | 708.70 | 695.17 |
| 8 | fluoromethane | C1s | 293.56 | 1 | 278.97 | 296.38 | 303.48 | 303.48 | 296.38 |
| 9 | trifluoromethane | F1s | 694.1 | 0 1 2 | 672.91 | 690.87 | 696.80 | 710.44 | 696.99 |
| 9 | trifluoromethane | C1s | 299.16 | 3 | 284.04 | 302.06 | 308.56 | 308.56 | 302.06 |
| 10 | methanol | O1s | 538.88 | 0 | 520.57 | 543.46 | 554.81 | 554.81 | 541.80 |
| 10 | methanol | C1s | 292.3 | 1 | 278.09 | 295.29 | 302.62 | 302.62 | 295.28 |
| 11 | formaldehyde | O1s | 539.33 | 0 | 521.23 | 543.78 | 555.39 | 555.39 | 542.12 |
| 11 | formaldehyde | C1s | 294.38 | 1 | 279.81 | 297.41 | 304.29 | 304.29 | 297.47 |
| 12 | dimethylether | O1s | 538.36 | 0 | 520.67 | 542.92 | 554.81 | 554.81 | 541.32 |
| 12 | dimethylether | C1s | 292.17 | 1 2 | 278.06 | 294.96 | 302.38 | 302.57 | 295.07 |
| 13 | formicacid | O1s(OH) | 540.69 | 0 | 522.46 | 545.06 | 556.62 | 556.62 | 543.44 |
| 13 | formicacid | O1s(C=O) | 539.02 | 1 | 520.91 | 543.25 | 555.09 | 555.09 | 541.60 |
| 13 | formicacid | C1s | 295.75 | 2 | 280.97 | 298.64 | 305.45 | 305.45 | 298.72 |
| 14 | acetone | O1s | 537.73 | 0 | 520.32 | 542.24 | 554.47 | 554.47 | 540.58 |
| 14 | acetone | C1s(C=O) | 293.88 | 1 | 279.51 | 296.56 | 304.00 | 304.00 | 296.61 |
| 14 | acetone | C1s(CH3) | 291.23 | 2 3 | 277.18 | 286.62 | 286.61 | 301.69 | 293.98 |
| 15 | methylformate | O1s(OCH3) | 539.64 | 0 | 522.23 | 544.24 | 556.34 | 556.34 | 542.68 |
| 15 | methylformate | O1s(C=O) | 538.24 | 1 | 520.66 | 542.79 | 554.82 | 554.82 | 541.14 |
| 16 | aceticacid | O1s(OH) | 540.1 | 0 | 522.09 | 544.49 | 556.24 | 556.24 | 542.88 |
| 16 | aceticacid | O1s(C=O) | 538.31 | 1 | 520.44 | 542.55 | 554.61 | 554.61 | 540.91 |
| 16 | aceticacid | C1s(COOH) | 295.35 | 2 | 280.81 | 298.20 | 305.30 | 305.30 | 298.27 |
| 16 | aceticacid | C1s(CH3) | 291.55 | 3 | 277.46 | 294.41 | 301.98 | 301.98 | 294.41 |
| 17 | water | O1s | 539.7 | 0 | 520.65 | 544.24 | 555.00 | 555.00 | 542.53 |
| 18 | ozone | O1smiddle | 546.44 | 0 | 528.92 | 551.61 | 562.95 | 562.95 | 550.16 |

TABLE S2 continued:

| index | mol | core level | Ref. | orbital | DFA | GSC2 | GSC | LOSC2 | lrLOSC |
|---|---|---|---|---|---|---|---|---|---|
| 18 | ozone | O1sterminal | 541.75 | 1 2 | 524.07 | 538.83 | 539.32 | 558.21 | 544.72 |
| 19 | oxygen | O1sweaker | 544.2 | 0 | 524.99 | 539.97 | 539.49 | 559.12 | 547.08 |
| 19 | oxygen | O1sstronger | 543.1 | 1 | 524.98 | 539.97 | 539.49 | 559.11 | 547.08 |
| 20 | nitrogen | N1s | 409.93 | 0 1 | 392.59 | 405.45 | 404.98 | 421.44 | 412.85 |
| 21 | ammonia | N1s | 405.52 | 0 | 389.11 | 408.39 | 417.95 | 417.95 | 408.39 |
| 22 | hydrogencyanide | N1s | 406.8 | 0 | 390.49 | 409.65 | 419.33 | 419.33 | 409.65 |
| 22 | hydrogencyanide | C1s | 293.5 | 1 | 278.56 | 296.26 | 303.05 | 303.05 | 296.26 |
| 23 | acetonitrile | N1s | 405.58 | 0 | 389.73 | 408.44 | 418.58 | 418.58 | 408.44 |
| 23 | acetonitrile | C1s(CH3) | 292.88 | 1 | 278.48 | 295.55 | 302.97 | 302.99 | 295.57 |
| 23 | acetonitrile | C1s(CN) | 292.6 | 2 | 278.17 | 295.56 | 302.65 | 302.66 | 295.56 |
| 24 | glycine | O1s(OH) | 540.2 | 0 | 522.17 | 544.54 | 556.31 | 556.31 | 542.94 |
| 24 | glycine | O1s(C=O) | 538.4 | 1 | 520.64 | 542.65 | 554.80 | 554.80 | 541.01 |
| 24 | glycine | N1s | 405.4 | 2 | 389.50 | 408.31 | 418.36 | 418.36 | 408.31 |
| 24 | glycine | C1s(COOH) | 295.2 | 3 | 280.76 | 298.01 | 305.24 | 305.24 | 298.08 |
| 24 | glycine | C1s(CH2) | 292.3 | 4 | 278.29 | 295.13 | 302.81 | 302.81 | 295.12 |
| 25 | pyridine | N1s | 404.82 | 0 | 389.69 | 407.60 | 418.54 | 418.54 | 407.60 |
| 26 | pyrrole | N1s | 406.18 | 0 | 390.89 | 408.99 | 419.74 | 419.74 | 408.99 |
| 27 | aniline | N1s | 405.31 | 0 | 389.89 | 408.03 | 418.74 | 418.74 | 408.03 |
| 28 | urea | O1s | 537.19 | 0 | 519.48 | 541.43 | 553.65 | 553.65 | 539.76 |
| 28 | urea | N1s | 406.09 | 1 2 | 390.26 | 401.16 | 402.02 | 419.11 | 408.93 |
| 28 | urea | C1s | 294.84 | 3 | 280.41 | 297.80 | 304.90 | 304.90 | 297.84 |
| 29 | methylamine | N1s | 405.17 | 0 | 389.11 | 408.00 | 417.96 | 417.96 | 408.00 |
| 31 | benzene | C1s | 290.38 | 0 1 2 3 4 5 | 277.08 | 282.53 | 279.77 | 301.58 | 293.17 |

Table S3: Absolute CLBEs of systems from CORE65 test set.[S1] The calculations were performed with def2-TZVP/PBE using QM4D.[S2]

| index | mol | core level | Ref. | orbital | DFA | GSC2 | GSC | LOSC2 | lrLOSC |
|---|---|---|---|---|---|---|---|---|---|
| 1 | methane | C1s | 290.84 | 0 | 268.54 | 293.27 | 299.15 | 299.15 | 293.27 |
| 2 | ethane | C1s | 290.71 | 0 1 | 268.71 | 282.72 | 281.43 | 299.32 | 293.21 |
| 3 | ethene | C1s | 290.82 | 0 1 | 269.07 | 283.47 | 282.14 | 299.68 | 293.36 |
| 4 | ethyne | C1s | 291.25 | 0 1 | 269.30 | 284.09 | 282.65 | 299.90 | 293.77 |

TABLE S3 continued:

| index | mol | core level | Ref. | orbital | DFA | GSC2 | GSC | LOSC2 | lrLOSC |
|---|---|---|---|---|---|---|---|---|---|
| 5 | carbonmonoxide | O1s | 542.1 | 0 | 513.23 | 546.86 | 555.59 | 555.60 | 545.31 |
| 5 | carbonmonoxide | C1s | 296.23 | 1 | 272.18 | 298.25 | 302.74 | 302.74 | 298.34 |
| 6 | carbondioxide | O1s | 541.32 | 0 1 | 512.54 | 545.26 | 554.37 | 554.83 | 544.10 |
| 6 | carbondioxide | C1s | 297.7 | 2 | 273.81 | 299.63 | 304.37 | 304.37 | 299.72 |
| 7 | tetrafluoromethane | F1s | 695.2 | 0 1 2 3 | 661.89 | 681.08 | 679.00 | 708.78 | 697.76 |
| 7 | tetrafluoromethane | C1s | 301.9 | 4 | 278.01 | 303.82 | 308.65 | 308.65 | 303.82 |
| 8 | fluoromethane | F1s | 692.4 | 0 | 659.59 | 695.29 | 706.49 | 706.49 | 695.29 |
| 8 | fluoromethane | C1s | 293.56 | 1 | 270.93 | 295.94 | 301.54 | 301.54 | 295.94 |
| 9 | trifluoromethane | F1s | 694.1 | 0 1 2 | 661.22 | 695.53 | 705.65 | 708.12 | 696.94 |
| 9 | trifluoromethane | C1s | 299.16 | 3 | 275.69 | 301.26 | 306.31 | 306.31 | 301.26 |
| 10 | methanol | O1s | 538.88 | 0 | 510.27 | 543.47 | 552.77 | 552.77 | 541.84 |
| 10 | methanol | C1s | 292.3 | 1 | 270.09 | 294.90 | 300.73 | 300.73 | 294.89 |
| 11 | formaldehyde | O1s | 539.33 | 0 | 510.91 | 543.84 | 553.33 | 553.33 | 542.22 |
| 11 | formaldehyde | C1s | 294.38 | 1 | 271.72 | 296.90 | 302.30 | 302.30 | 296.96 |
| 12 | dimethylether | O1s | 538.36 | 0 | 510.46 | 543.02 | 552.86 | 552.86 | 541.45 |
| 12 | dimethylether | C1s | 292.17 | 1 2 | 270.09 | 294.68 | 300.70 | 300.70 | 294.69 |
| 13 | formicacid | O1s(OH) | 540.69 | 0 | 512.12 | 545.01 | 554.53 | 554.53 | 543.43 |
| 13 | formicacid | O1s(C=O) | 539.02 | 1 | 510.55 | 543.21 | 552.98 | 552.98 | 541.60 |
| 13 | formicacid | C1s | 295.75 | 2 | 272.71 | 297.91 | 303.30 | 303.30 | 297.98 |
| 14 | acetone | O1s | 537.73 | 0 | 510.00 | 542.25 | 552.40 | 552.40 | 540.63 |
| 14 | acetone | C1s(C=O) | 293.88 | 1 | 271.46 | 296.08 | 302.05 | 302.05 | 296.13 |
| 14 | acetone | C1s(CH3) | 291.23 | 2 3 | 269.24 | 292.04 | 297.23 | 299.85 | 293.62 |
| 15 | methylformate | O1s(OCH3) | 539.64 | 0 | 511.98 | 544.30 | 554.34 | 554.34 | 542.77 |
| 15 | methylformate | O1s(C=O) | 538.24 | 1 | 510.31 | 542.76 | 552.73 | 552.73 | 541.15 |
| 16 | aceticacid | O1s(OH) | 540.1 | 0 | 511.74 | 544.42 | 554.15 | 554.15 | 542.85 |
| 16 | aceticacid | O1s(C=O) | 538.31 | 1 | 510.09 | 542.51 | 552.51 | 552.51 | 540.91 |
| 16 | aceticacid | C1s(COOH) | 295.35 | 2 | 272.59 | 297.51 | 303.18 | 303.18 | 297.58 |
| 16 | aceticacid | C1s(CH3) | 291.55 | 3 | 269.50 | 294.03 | 300.13 | 300.13 | 294.02 |
| 17 | water | O1s | 539.7 | 0 | 510.26 | 544.16 | 552.87 | 552.87 | 542.47 |
| 18 | ozone | O1smiddle | 546.44 | 0 | 518.15 | 551.28 | 560.44 | 560.44 | 549.87 |
| 18 | ozone | O1sterminal | 541.75 | 1 2 | 513.43 | 546.03 | 555.83 | 555.83 | 544.49 |
| 19 | oxygen | O1sweaker | 544.2 | 0 | 514.17 | 534.86 | 532.09 | 556.54 | 546.62 |
| 19 | oxygen | O1sstronger | 543.1 | 1 | 514.17 | 534.86 | 532.09 | 556.54 | 546.62 |

TABLE S3 continued:

| index | mol | core level | Ref. | orbital | DFA | GSC2 | GSC | LOSC2 | lrLOSC |
|---|---|---|---|---|---|---|---|---|---|
| 20 | nitrogen | N1s | 409.93 | 0 1 | 383.26 | 401.19 | 398.73 | 419.30 | 412.48 |
| 21 | ammonia | N1s | 405.52 | 0 | 379.98 | 408.24 | 416.02 | 416.02 | 408.24 |
| 22 | hydrogencyanide | N1s | 406.8 | 0 | 381.29 | 409.44 | 417.33 | 417.33 | 409.44 |
| 22 | hydrogencyanide | C1s | 293.5 | 1 | 270.54 | 295.81 | 301.13 | 301.13 | 295.81 |
| 23 | acetonitrile | N1s | 405.58 | 0 | 380.53 | 408.21 | 416.57 | 416.57 | 408.21 |
| 23 | acetonitrile | C1s(CH3) | 292.88 | 1 | 270.53 | 295.19 | 301.14 | 301.14 | 295.20 |
| 23 | acetonitrile | C1s(CN) | 292.6 | 2 | 270.16 | 295.12 | 300.75 | 300.75 | 295.12 |
| 24 | glycine | O1s(OH) | 540.2 | 0 | 511.81 | 544.45 | 554.21 | 554.21 | 542.88 |
| 24 | glycine | O1s(C=O) | 538.4 | 1 | 510.28 | 542.59 | 552.69 | 552.69 | 540.99 |
| 24 | glycine | N1s | 405.4 | 2 | 380.42 | 408.19 | 416.48 | 416.48 | 408.18 |
| 24 | glycine | C1s(COOH) | 295.2 | 3 | 272.52 | 297.30 | 303.11 | 303.11 | 297.36 |
| 24 | glycine | C1s(CH2) | 292.3 | 4 | 270.30 | 294.73 | 300.93 | 300.93 | 294.72 |
| 25 | pyridine | N1s | 404.82 | 0 | 380.62 | 407.53 | 416.66 | 416.66 | 407.53 |
| 26 | pyrrole | N1s | 406.18 | 0 | 381.87 | 409.00 | 417.90 | 417.91 | 409.00 |
| 27 | aniline | N1s | 405.31 | 0 | 380.89 | 407.98 | 416.93 | 416.93 | 407.98 |
| 28 | urea | O1s | 537.19 | 0 | 509.15 | 541.40 | 551.58 | 551.58 | 539.77 |
| 28 | urea | N1s | 406.09 | 1 2 | 381.14 | 408.64 | 416.99 | 417.19 | 408.76 |
| 28 | urea | C1s | 294.84 | 3 | 272.15 | 297.06 | 302.75 | 302.75 | 297.10 |
| 29 | methylamine | N1s | 405.17 | 0 | 380.05 | 407.92 | 416.09 | 416.09 | 407.92 |
| 31 | benzene | C1s | 290.38 | 0 1 2 3 4 5 | 269.19 | 276.88 | 272.54 | 299.79 | 292.89 |

Table S4: Relative CLBEs (in eV) of systems from CORE65 test set.[S1] The calculations were performed with def2-TZVP/BLYP on QM4D.[S2] The relative core-level binding energy is defined as the energy difference relative to a reference molecule, $\Delta E_{\text{relative}} = E_{\text{absolute}} - E_{\text{ref\_absolute}}$. $CH_4$, $NH_3$, $H_2O$ and $CH_3F$ are the reference molecules for C1s, N1s, O1s and F1s respectively.

| index | mol | core level | Ref. | orbital | DFA | GSC2 | GSC | LOSC2 | lrLOSC |
|---|---|---|---|---|---|---|---|---|---|
| 1 | methane | C1s | 0 | 0 | 0.00 | 0.00 | 0.00 | 0.00 | 0.00 |
| 2 | ethane | C1s | −0.13 | 0 1 | 0.13 | −10.51 | −17.75 | 0.13 | −0.12 |
| 3 | ethene | C1s | −0.02 | 0 1 | 0.48 | −9.77 | −17.06 | 0.48 | 0.03 |
| 4 | ethyne | C1s | 0.41 | 0 1 | 0.69 | −9.16 | −16.57 | 0.68 | 0.44 |
| 5 | carbonmonoxide | C1s | 5.39 | 1 | 3.65 | 5.04 | 3.60 | 3.60 | 5.13 |

TABLE S4 continued:

| index | mol | core level | Ref. | orbital | DFA | GSC2 | GSC | LOSC2 | lrLOSC |
|---|---|---|---|---|---|---|---|---|---|
| 6 | carbondioxide | C1s | 6.86 | 2 | 5.38 | 6.48 | 5.35 | 5.35 | 6.56 |
| 7 | tetrafluoromethane | C1s | 11.06 | 4 | 9.64 | 10.66 | 9.67 | 9.67 | 10.66 |
| 8 | fluoromethane | C1s | 2.72 | 1 | 2.42 | 2.68 | 2.43 | 2.43 | 2.68 |
| 9 | trifluoromethane | C1s | 8.32 | 3 | 7.26 | 8.07 | 7.29 | 7.29 | 8.07 |
| 10 | methanol | C1s | 1.46 | 1 | 1.57 | 1.63 | 1.60 | 1.60 | 1.62 |
| 11 | formaldehyde | C1s | 3.54 | 1 | 3.21 | 3.66 | 3.19 | 3.19 | 3.72 |
| 12 | dimethylether | C1s | 1.33 | 1 2 | 1.55 | 1.39 | 1.55 | 1.56 | 1.40 |
| 13 | formicacid | C1s | 4.91 | 2 | 4.24 | 4.69 | 4.23 | 4.23 | 4.77 |
| 22 | hydrogencyanide | C1s | 2.66 | 1 | 1.99 | 2.54 | 1.98 | 1.98 | 2.54 |
| 28 | urea | C1s | 4 | 3 | 3.66 | 3.80 | 3.66 | 3.66 | 3.84 |
| 31 | benzene | C1s | −0.46 | 0 1 2 3 4 5 | 0.54 | −16.38 | −26.71 | 0.54 | −0.51 |
| 14 | acetone | C1s(C=O) | 3.04 | 1 | 2.88 | 2.73 | 2.86 | 2.86 | 2.78 |
| 24 | glycine | C1s(CH2) | 1.46 | 4 | 1.74 | 1.40 | 1.76 | 1.76 | 1.39 |
| 14 | acetone | C1s(CH3) | 0.39 | 2 3 | 0.67 | −0.03 | 0.12 | 0.68 | 0.31 |
| 16 | aceticacid | C1s(CH3) | 0.71 | 3 | 0.94 | 0.73 | 0.97 | 0.97 | 0.72 |
| 23 | acetonitrile | C1s(CH3) | 2.04 | 1 | 1.97 | 1.88 | 1.96 | 1.97 | 1.88 |
| 23 | acetonitrile | C1s(CN) | 1.76 | 2 | 1.57 | 1.80 | 1.56 | 1.56 | 1.80 |
| 16 | aceticacid | C1s(COOH) | 4.51 | 2 | 4.08 | 4.23 | 4.06 | 4.06 | 4.30 |
| 24 | glycine | C1s(COOH) | 4.36 | 3 | 4.01 | 4.02 | 4.00 | 4.00 | 4.09 |
| 7 | tetrafluoromethane | F1s | 2.8 | 0 1 2 3 | 2.33 | 2.51 | 2.32 | 2.33 | 2.52 |
| 8 | fluoromethane | F1s | 0 | 0 | 0.00 | 0.00 | 0.00 | 0.00 | 0.00 |
| 9 | trifluoromethane | F1s | 1.7 | 0 1 2 | 1.66 | 1.66 | 1.63 | 1.66 | 1.68 |
| 20 | nitrogen | N1s | 4.41 | 0 1 | 3.32 | −6.94 | −17.25 | 3.31 | 4.28 |
| 21 | ammonia | N1s | 0 | 0 | 0.00 | 0.00 | 0.00 | 0.00 | 0.00 |
| 22 | hydrogencyanide | N1s | 1.28 | 0 | 1.28 | 1.17 | 1.27 | 1.27 | 1.17 |
| 23 | acetonitrile | N1s | 0.06 | 0 | 0.51 | −0.07 | 0.51 | 0.51 | −0.07 |
| 24 | glycine | N1s | −0.12 | 2 | 0.37 | −0.13 | 0.39 | 0.39 | −0.14 |
| 25 | pyridine | N1s | −0.7 | 0 | 0.51 | −0.87 | 0.51 | 0.51 | −0.87 |
| 26 | pyrrole | N1s | 0.66 | 0 | 1.74 | 0.57 | 1.73 | 1.73 | 0.57 |
| 27 | aniline | N1s | −0.21 | 0 | 0.81 | −0.37 | 0.81 | 0.81 | −0.37 |
| 28 | urea | N1s | 0.57 | 1 2 | 1.11 | 0.45 | 1.11 | 1.11 | 0.46 |
| 29 | methylamine | N1s | −0.35 | 0 | 0.00 | −0.40 | 0.00 | 0.00 | −0.40 |
| 5 | carbonmonoxide | O1s | 2.4 | 0 | 2.93 | 2.64 | 2.67 | 2.67 | 2.77 |

TABLE S4 continued:

| index | mol | core level | Ref. | orbital | DFA | GSC2 | GSC | LOSC2 | lrLOSC |
|---|---|---|---|---|---|---|---|---|---|
| 6 | carbondioxide | O1s | 1.62 | 0 1 | 2.23 | 1.09 | 1.57 | 1.90 | 1.56 |
| 10 | methanol | O1s | −0.82 | 0 | −0.07 | −0.78 | −0.19 | −0.19 | −0.73 |
| 11 | formaldehyde | O1s | −0.37 | 0 | 0.59 | −0.41 | 0.39 | 0.39 | −0.34 |
| 12 | dimethylether | O1s | −1.34 | 0 | 0.05 | −1.32 | −0.18 | −0.18 | −1.20 |
| 14 | acetone | O1s | −1.97 | 0 | −0.33 | −2.00 | −0.55 | −0.55 | −1.93 |
| 17 | water | O1s | 0 | 0 | 0.00 | 0.00 | 0.00 | 0.00 | 0.00 |
| 28 | urea | O1s | −2.51 | 0 | −1.17 | −2.84 | −1.37 | −1.37 | −2.78 |
| 13 | formicacid | O1s(C=O) | −0.68 | 1 | 0.24 | −1.02 | 0.05 | 0.05 | −0.94 |
| 15 | methylformate | O1s(C=O) | −1.46 | 1 | −0.02 | −1.49 | −0.23 | −0.22 | −1.40 |
| 16 | aceticacid | O1s(C=O) | −1.39 | 1 | −0.23 | −1.72 | −0.43 | −0.42 | −1.64 |
| 24 | glycine | O1s(C=O) | −1.3 | 1 | −0.04 | −1.64 | −0.24 | −0.24 | −1.55 |
| 15 | methylformate | O1s(OCH3) | −0.06 | 0 | 1.58 | −0.02 | 1.32 | 1.31 | 0.14 |
| 13 | formicacid | O1s(OH) | 0.99 | 0 | 1.79 | 0.76 | 1.58 | 1.58 | 0.87 |
| 16 | aceticacid | O1s(OH) | 0.4 | 0 | 1.41 | 0.18 | 1.19 | 1.19 | 0.29 |
| 24 | glycine | O1s(OH) | 0.5 | 0 | 1.48 | 0.21 | 1.26 | 1.26 | 0.33 |
| 18 | ozone | O1smiddle | 6.74 | 0 | 7.81 | 6.99 | 7.49 | 7.49 | 7.26 |
| 19 | oxygen | O1sstronger | 3.4 | 1 | 3.92 | −8.42 | −19.16 | 3.67 | 4.13 |
| 18 | ozone | O1sterminal | 2.05 | 1 2 | 3.17 | −11.19 | −22.86 | 2.96 | 1.99 |
| 19 | oxygen | O1sweaker | 4.5 | 0 | 3.92 | −8.42 | −19.16 | 3.67 | 4.14 |

Table S5: Relative CLBEs (in eV) of systems from CORE65 test set.[S1] The calculations were perfromed with def2-TZVP/B3LYP on QM4D.[S2] The relative core-level binding energy is defined as the energy difference relative to a reference molecule, $\Delta E_{\text{relative}} = E_{\text{absolute}} - E_{\text{ref\_absolute}}$. $CH_4$, $NH_3$, $H_2O$ and $CH_3F$ are the reference molecules for C1s, N1s, O1s and F1s respectively.

| index | mol | core level | Ref. | orbital | DFA | GSC2 | GSC | LOSC2 | lrLOSC |
|---|---|---|---|---|---|---|---|---|---|
| 1 | methane | C1s | 0 | 0 | 0.00 | 0.00 | 0.00 | 0.00 | 0.00 |
| 2 | ethane | C1s | −0.13 | 0 1 | 0.14 | −7.24 | −14.17 | 0.15 | −0.10 |
| 3 | ethene | C1s | −0.02 | 0 1 | 0.53 | −6.52 | −13.51 | 0.53 | 0.05 |
| 4 | ethyne | C1s | 0.41 | 0 1 | 0.76 | −5.94 | −13.06 | 0.76 | 0.50 |
| 5 | carbonmonoxide | C1s | 5.39 | 1 | 3.83 | 5.31 | 3.79 | 3.79 | 5.40 |
| 6 | carbondioxide | C1s | 6.86 | 2 | 5.80 | 7.03 | 5.77 | 5.77 | 7.12 |

TABLE S5 continued:

| index | mol | core level | Ref. | orbital | DFA | GSC2 | GSC | LOSC2 | lrLOSC |
|---|---|---|---|---|---|---|---|---|---|
| 7 | tetrafluoromethane | C1s | 11.06 | 4 | 10.08 | 11.21 | 10.11 | 10.11 | 11.21 |
| 8 | fluoromethane | C1s | 2.72 | 1 | 2.51 | 2.79 | 2.51 | 2.51 | 2.79 |
| 9 | trifluoromethane | C1s | 8.32 | 3 | 7.58 | 8.46 | 7.60 | 7.60 | 8.46 |
| 10 | methanol | C1s | 1.46 | 1 | 1.63 | 1.69 | 1.65 | 1.65 | 1.69 |
| 11 | formaldehyde | C1s | 3.54 | 1 | 3.34 | 3.81 | 3.32 | 3.32 | 3.87 |
| 12 | dimethylether | C1s | 1.33 | 1 2 | 1.60 | 1.36 | 1.42 | 1.60 | 1.47 |
| 13 | formicacid | C1s | 4.91 | 2 | 4.50 | 5.04 | 4.49 | 4.49 | 5.12 |
| 22 | hydrogencyanide | C1s | 2.66 | 1 | 2.09 | 2.66 | 2.09 | 2.09 | 2.66 |
| 28 | urea | C1s | 4 | 3 | 3.95 | 4.20 | 3.94 | 3.94 | 4.24 |
| 31 | benzene | C1s | −0.46 | 0 1 2 3 4 5 | 0.62 | −11.07 | −21.19 | 0.62 | −0.43 |
| 14 | acetone | C1s(C=O) | 3.04 | 1 | 3.05 | 2.96 | 3.03 | 3.03 | 3.01 |
| 24 | glycine | C1s(CH2) | 1.46 | 4 | 1.83 | 1.53 | 1.85 | 1.85 | 1.52 |
| 14 | acetone | C1s(CH3) | 0.39 | 2 3 | 0.72 | −6.98 | −14.35 | 0.72 | 0.39 |
| 16 | aceticacid | C1s(CH3) | 0.71 | 3 | 1.00 | 0.82 | 1.02 | 1.02 | 0.81 |
| 23 | acetonitrile | C1s(CH3) | 2.04 | 1 | 2.02 | 1.95 | 2.01 | 2.02 | 1.97 |
| 23 | acetonitrile | C1s(CN) | 1.76 | 2 | 1.71 | 1.96 | 1.68 | 1.70 | 1.96 |
| 16 | aceticacid | C1s(COOH) | 4.51 | 2 | 4.35 | 4.60 | 4.33 | 4.33 | 4.67 |
| 24 | glycine | C1s(COOH) | 4.36 | 3 | 4.30 | 4.41 | 4.28 | 4.28 | 4.48 |
| 7 | tetrafluoromethane | F1s | 2.8 | 0 1 2 3 | 2.48 | −8.55 | −21.93 | 2.48 | 2.72 |
| 8 | fluoromethane | F1s | 0 | 0 | 0.00 | 0.00 | 0.00 | 0.00 | 0.00 |
| 9 | trifluoromethane | F1s | 1.7 | 0 1 2 | 1.74 | −4.30 | −11.90 | 1.74 | 1.82 |
| 20 | nitrogen | N1s | 4.41 | 0 1 | 3.49 | −2.94 | −12.98 | 3.48 | 4.46 |
| 21 | ammonia | N1s | 0 | 0 | 0.00 | 0.00 | 0.00 | 0.00 | 0.00 |
| 22 | hydrogencyanide | N1s | 1.28 | 0 | 1.38 | 1.25 | 1.38 | 1.38 | 1.25 |
| 23 | acetonitrile | N1s | 0.06 | 0 | 0.62 | 0.04 | 0.62 | 0.62 | 0.04 |
| 24 | glycine | N1s | −0.12 | 2 | 0.39 | −0.08 | 0.41 | 0.41 | −0.09 |
| 25 | pyridine | N1s | −0.7 | 0 | 0.58 | −0.79 | 0.58 | 0.58 | −0.79 |
| 26 | pyrrole | N1s | 0.66 | 0 | 1.78 | 0.59 | 1.78 | 1.78 | 0.59 |
| 27 | aniline | N1s | −0.21 | 0 | 0.78 | −0.36 | 0.78 | 0.78 | −0.36 |
| 28 | urea | N1s | 0.57 | 1 2 | 1.15 | −7.23 | −15.93 | 1.15 | 0.54 |
| 29 | methylamine | N1s | −0.35 | 0 | 0.00 | −0.39 | 0.00 | 0.00 | −0.39 |
| 5 | carbonmonoxide | O1s | 2.4 | 0 | 2.95 | 2.64 | 2.72 | 2.72 | 2.75 |
| 6 | carbondioxide | O1s | 1.62 | 0 1 | 2.33 | −7.39 | −18.73 | 2.03 | 1.63 |

TABLE S5 continued:

| index | mol | core level | Ref. | orbital | DFA | GSC2 | GSC | LOSC2 | lrLOSC |
|---|---|---|---|---|---|---|---|---|---|
| 10 | methanol | O1s | −0.82 | 0 | −0.08 | −0.78 | −0.19 | −0.19 | −0.73 |
| 11 | formaldehyde | O1s | −0.37 | 0 | 0.57 | −0.45 | 0.40 | 0.40 | −0.41 |
| 12 | dimethylether | O1s | −1.34 | 0 | 0.01 | −1.32 | −0.19 | −0.19 | −1.21 |
| 14 | acetone | O1s | −1.97 | 0 | −0.34 | −2.00 | −0.53 | −0.53 | −1.94 |
| 17 | water | O1s | 0 | 0 | 0.00 | 0.00 | 0.00 | 0.00 | 0.00 |
| 28 | urea | O1s | −2.51 | 0 | −1.17 | −2.80 | −1.34 | −1.34 | −2.76 |
| 13 | formicacid | O1s(C=O) | −0.68 | 1 | 0.26 | −0.99 | 0.09 | 0.09 | −0.93 |
| 15 | methylformate | O1s(C=O) | −1.46 | 1 | 0.00 | −1.44 | −0.18 | −0.18 | −1.38 |
| 16 | aceticacid | O1s(C=O) | −1.39 | 1 | −0.21 | −1.69 | −0.38 | −0.38 | −1.62 |
| 24 | glycine | O1s(C=O) | −1.3 | 1 | −0.01 | −1.59 | −0.20 | −0.20 | −1.51 |
| 15 | methylformate | O1s(OCH3) | −0.06 | 0 | 1.58 | 0.01 | 1.34 | 1.34 | 0.15 |
| 13 | formicacid | O1s(OH) | 0.99 | 0 | 1.80 | 0.82 | 1.62 | 1.62 | 0.91 |
| 16 | aceticacid | O1s(OH) | 0.4 | 0 | 1.43 | 0.25 | 1.24 | 1.24 | 0.36 |
| 24 | glycine | O1s(OH) | 0.5 | 0 | 1.52 | 0.30 | 1.32 | 1.32 | 0.41 |
| 18 | ozone | O1smiddle | 6.74 | 0 | 8.26 | 7.37 | 7.95 | 7.95 | 7.63 |
| 19 | oxygen | O1sstronger | 3.4 | 1 | 4.33 | −4.27 | −15.51 | 4.11 | 4.55 |
| 18 | ozone | O1sterminal | 2.05 | 1 2 | 3.41 | −5.40 | −15.68 | 3.22 | 2.19 |
| 19 | oxygen | O1sweaker | 4.5 | 0 | 4.34 | −4.26 | −15.51 | 4.12 | 4.55 |

Table S6: Relative CLBEs (in eV) of systems from CORE65 test set.[S1] The calculations were performed with def2-TZVP/PBE on QM4D.[S2] The relative core-level binding energy is defined as the energy difference relative to a reference molecule, $\Delta E_{\text{relative}} = E_{\text{absolute}} - E_{\text{ref\_absolute}}$. $CH_4$, $NH_3$, $H_2O$ and $CH_3F$ are the reference molecules for C1s, N1s, O1s and F1s respectively.

| index | mol | core level | Ref. | orbital | DFA | GSC2 | GSC | LOSC2 | lrLOSC |
|---|---|---|---|---|---|---|---|---|---|
| 1 | methane | C1s | 0 | 0 | 0.00 | 0.00 | 0.00 | 0.00 | 0.00 |
| 2 | ethane | C1s | −0.13 | 0 1 | 0.17 | −10.55 | −17.71 | 0.18 | −0.06 |
| 3 | ethene | C1s | −0.02 | 0 1 | 0.54 | −9.80 | −17.00 | 0.53 | 0.10 |
| 4 | ethyne | C1s | 0.41 | 0 1 | 0.76 | −9.18 | −16.50 | 0.75 | 0.50 |
| 5 | carbonmonoxide | C1s | 5.39 | 1 | 3.65 | 4.98 | 3.60 | 3.60 | 5.08 |
| 6 | carbondioxide | C1s | 6.86 | 2 | 5.27 | 6.36 | 5.23 | 5.23 | 6.45 |
| 7 | tetrafluoromethane | C1s | 11.06 | 4 | 9.47 | 10.55 | 9.50 | 9.50 | 10.55 |

TABLE S6 continued:

| index | mol | core level | Ref. | orbital | DFA | GSC2 | GSC | LOSC2 | lrLOSC |
|---|---|---|---|---|---|---|---|---|---|
| 8 | fluoromethane | C1s | 2.72 | 1 | 2.39 | 2.67 | 2.40 | 2.40 | 2.67 |
| 9 | trifluoromethane | C1s | 8.32 | 3 | 7.15 | 7.99 | 7.17 | 7.17 | 7.99 |
| 10 | methanol | C1s | 1.46 | 1 | 1.56 | 1.63 | 1.59 | 1.59 | 1.62 |
| 11 | formaldehyde | C1s | 3.54 | 1 | 3.18 | 3.64 | 3.16 | 3.16 | 3.69 |
| 12 | dimethylether | C1s | 1.33 | 1 2 | 1.55 | 1.41 | 1.56 | 1.56 | 1.42 |
| 13 | formicacid | C1s | 4.91 | 2 | 4.17 | 4.64 | 4.15 | 4.15 | 4.71 |
| 22 | hydrogencyanide | C1s | 2.66 | 1 | 2.00 | 2.54 | 1.98 | 1.98 | 2.54 |
| 28 | urea | C1s | 4 | 3 | 3.61 | 3.80 | 3.60 | 3.60 | 3.84 |
| 31 | benzene | C1s | −0.46 | 0 1 2 3 4 5 | 0.65 | −16.39 | −26.61 | 0.65 | −0.37 |
| 14 | acetone | C1s(C=O) | 3.04 | 1 | 2.92 | 2.82 | 2.90 | 2.90 | 2.86 |
| 24 | glycine | C1s(CH2) | 1.46 | 4 | 1.77 | 1.46 | 1.79 | 1.79 | 1.45 |
| 14 | acetone | C1s(CH3) | 0.39 | 2 3 | 0.70 | −1.23 | −1.91 | 0.71 | 0.35 |
| 16 | aceticacid | C1s(CH3) | 0.71 | 3 | 0.96 | 0.76 | 0.98 | 0.98 | 0.75 |
| 23 | acetonitrile | C1s(CH3) | 2.04 | 1 | 2.00 | 1.92 | 1.99 | 2.00 | 1.93 |
| 23 | acetonitrile | C1s(CN) | 1.76 | 2 | 1.62 | 1.85 | 1.60 | 1.61 | 1.85 |
| 16 | aceticacid | C1s(COOH) | 4.51 | 2 | 4.05 | 4.24 | 4.03 | 4.03 | 4.31 |
| 24 | glycine | C1s(COOH) | 4.36 | 3 | 3.98 | 4.03 | 3.96 | 3.96 | 4.09 |
| 7 | tetrafluoromethane | F1s | 2.8 | 0 1 2 3 | 2.29 | −14.22 | −27.48 | 2.29 | 2.47 |
| 8 | fluoromethane | F1s | 0 | 0 | 0.00 | 0.00 | 0.00 | 0.00 | 0.00 |
| 9 | trifluoromethane | F1s | 1.7 | 0 1 2 | 1.63 | 0.24 | −0.84 | 1.63 | 1.65 |
| 20 | nitrogen | N1s | 4.41 | 0 1 | 3.28 | −7.05 | −17.29 | 3.27 | 4.24 |
| 21 | ammonia | N1s | 0 | 0 | 0.00 | 0.00 | 0.00 | 0.00 | 0.00 |
| 22 | hydrogencyanide | N1s | 1.28 | 0 | 1.31 | 1.20 | 1.30 | 1.30 | 1.20 |
| 23 | acetonitrile | N1s | 0.06 | 0 | 0.55 | −0.03 | 0.54 | 0.54 | −0.03 |
| 24 | glycine | N1s | −0.12 | 2 | 0.44 | −0.05 | 0.46 | 0.46 | −0.06 |
| 25 | pyridine | N1s | −0.7 | 0 | 0.64 | −0.71 | 0.63 | 0.63 | −0.71 |
| 26 | pyrrole | N1s | 0.66 | 0 | 1.88 | 0.76 | 1.88 | 1.88 | 0.76 |
| 27 | aniline | N1s | −0.21 | 0 | 0.91 | −0.26 | 0.91 | 0.91 | −0.26 |
| 28 | urea | N1s | 0.57 | 1 2 | 1.16 | 0.40 | 0.96 | 1.16 | 0.52 |
| 29 | methylamine | N1s | −0.35 | 0 | 0.07 | −0.32 | 0.07 | 0.07 | −0.32 |
| 5 | carbonmonoxide | O1s | 2.4 | 0 | 2.97 | 2.71 | 2.72 | 2.72 | 2.83 |
| 6 | carbondioxide | O1s | 1.62 | 0 1 | 2.28 | 1.10 | 1.50 | 1.96 | 1.63 |
| 10 | methanol | O1s | −0.82 | 0 | 0.01 | −0.68 | −0.10 | −0.11 | −0.63 |

TABLE S6 continued:

| index | mol | core level | Ref. | orbital | DFA | GSC2 | GSC | LOSC2 | lrLOSC |
|---|---|---|---|---|---|---|---|---|---|
| 11 | formaldehyde | O1s | −0.37 | 0 | 0.65 | −0.32 | 0.46 | 0.46 | −0.26 |
| 12 | dimethylether | O1s | −1.34 | 0 | 0.20 | −1.14 | −0.01 | −0.01 | −1.02 |
| 14 | acetone | O1s | −1.97 | 0 | −0.26 | −1.91 | −0.47 | −0.47 | −1.84 |
| 17 | water | O1s | 0 | 0 | 0.00 | 0.00 | 0.00 | 0.00 | 0.00 |
| 28 | urea | O1s | −2.51 | 0 | −1.11 | −2.75 | −1.30 | −1.30 | −2.70 |
| 13 | formicacid | O1s(C=O) | −0.68 | 1 | 0.29 | −0.95 | 0.11 | 0.11 | −0.87 |
| 15 | methylformate | O1s(C=O) | −1.46 | 1 | 0.05 | −1.40 | −0.15 | −0.15 | −1.32 |
| 16 | aceticacid | O1s(C=O) | −1.39 | 1 | −0.17 | −1.65 | −0.36 | −0.36 | −1.57 |
| 24 | glycine | O1s(C=O) | −1.3 | 1 | 0.02 | −1.56 | −0.18 | −0.18 | −1.48 |
| 15 | methylformate | O1s(OCH3) | −0.06 | 0 | 1.72 | 0.15 | 1.47 | 1.47 | 0.30 |
| 13 | formicacid | O1s(OH) | 0.99 | 0 | 1.86 | 0.85 | 1.66 | 1.66 | 0.95 |
| 16 | aceticacid | O1s(OH) | 0.4 | 0 | 1.48 | 0.27 | 1.27 | 1.27 | 0.37 |
| 24 | glycine | O1s(OH) | 0.5 | 0 | 1.55 | 0.29 | 1.34 | 1.34 | 0.41 |
| 18 | ozone | O1smiddle | 6.74 | 0 | 7.89 | 7.13 | 7.57 | 7.57 | 7.40 |
| 19 | oxygen | O1sstronger | 3.4 | 1 | 3.91 | −9.30 | −20.79 | 3.67 | 4.14 |
| 18 | ozone | O1sterminal | 2.05 | 1 2 | 3.17 | 1.88 | 2.96 | 2.96 | 2.02 |
| 19 | oxygen | O1sweaker | 4.5 | 0 | 3.91 | −9.30 | −20.78 | 3.67 | 4.14 |

# References


(S1) Golze, D.; Keller, L.; Rinke, P. Accurate absolute and relative core-level binding energies from GW. *J. Phys. Chem. Lett.* **2020**, *11*, 1840–1847.

(S2) An in-house program for QM/MM simulations; available from `https://qm4d.org/`.
